# Supplementary material for: Offline Skill Generalization via Task and Motion Planning
Source: arXiv:2311.14328 source file (2023-11-24)
Supplement: Supplementary file 1 [file appendix.tex]

\section{Appendix}

% TODO: mention kinematic graphs (ref. integrated TAMP)

%%%%%%%%%%%%%%%%%%%%%%%%%%%%%%%%%%%%%%%%%%%%%%%%%%%%%%%%%%%%%%%%%%%%%%%%%%%%%%%%%%%%%%%%%%%%%%%%%%%%%%%%%
`stream.pddl`

; a stream that samples a gripper pose that allows it to push an object; similar to `sample-grasp`
  (:stream sample-align
    :inputs (?o ?p1 ?p2)
    :domain (and (Alignable ?o) (Pose ?o ?p1) (Pose ?o ?p2))
    :outputs (?g)
    :certified (Alignment ?o ?p1 ?p2 ?g)
  )

; a stream that generates a collision-free push trajectory; similar to `plan-base-motion`
  (:stream plan-push-motion
    :inputs (?a ?o ?p1 ?p2 ?g ?q1 ?q2)
    :domain (and (Controllable ?a) (Alignment ?o ?p1 ?p2 ?g) (Pose ?o ?p1) (AConf ?a ?q2) (BConf ?q1))
    :outputs (?t)
    :certified (and (ATraj ?t) (ArmMotion ?a ?p1 ?p2 ?q1 ?q2 ?t))
  )

%%%%%%%%%%%%%%%%%%%%%%%%%%%%%%%%%%%%%%%%%%%%%%%%%%%%%%%%%%%%%%%%%%%%%%%%%%%%%%%%%%%%%%%%%%%%%%%%%%%%%%%%%
`domain.pddl`

// extra predicates for accommodating pushing
  (:predicates
    (Kin2 ?a ?o ?p1 ?p2 ?g ?q1 ?q2 ?t) ; similar to `Kin` but additionally includes desired object pose `p2` and arm configuration `q2`
    (AtPush ?a ?o ?p ?g ?q) ; similar to `Grasp` but additionally includes desired object pose `p` and arm configuration `q`
    (ArmMotion ?a ?p1 ?p2 ?q1 ?q2 ?t) ; similar to `BaseMotion` but for the arm trajectory
  )
% Q: doesn't Kin2 do the same thing as AtPush and ArmMotion combined?
% A: no because Kin2 also plans for the base configuration, but for pushing we don't want the base to move

// action costs
(:functions
    (AlignCost)
    (PushCost)
)

; an action that places the gripper in a state that can push the object
; similar to `pick` action but has 2 extra parameters: p2 - goal object pose, q1 - arm configuration
  (:action align
    :parameters (?a ?o ?p1 ?p2 ?g ?q0 ?q2 ?t)
    :precondition (and (Kin2 ?a ?o ?p1 ?p2 ?g ?q0 ?q2 ?t)
                       (AtPose ?o ?p1)
                       (HandEmpty ?a)
                       (AtBConf ?q0)
                       (not (UnsafePose ?o ?p2)) ;the goal pose must be collision-free
                       (not (UnsafeAlignment ?o ?p1 ?p2 ?g))
                       (not (UnsafeATraj ?t))
                  )
    :effect (and (not (CanMove)) (AtPush ?a ?o ?p2 ?g ?q2) (AtAConf ?a ?q2)
                 (increase (total-cost) (AlignCost)))
  )

; push action
  (:action push
    :parameters (?a ?o ?p1 ?p2 ?g ?q0 ?q1 ?t)
    :precondition (and (ArmMotion ?a ?p1 ?p2 ?q0 ?q1 ?t)
                       (AtPush ?a ?o ?p2 ?g ?q1)
                       (AtAConf ?a ?q1)
                       (AtBConf ?q0)
                       (not (UnsafeATraj ?t))
                       (HandEmpty ?a)
                       (AtPose ?o ?p1)
                  )
    :effect (and (AtPose ?o ?p2) (CanMove)
                 (not (AtPush ?a ?o ?p2 ?g ?q1))
                 (not (AtAConf ?a ?q1))
                 (increase (total-cost) (PushCost)))
  )
